# Supplementary material for: Maximal Structuring of Acyclic Process Models
Source: arXiv:1108.2384 source file (2011-08-11)
Supplement: Supplementary file 1 [file appendix.tex]

\section{Appendix}
\label{apx:A}
%%%%%%%%%%%%%%%%%%%%%%%%%%%%%%%%%%%%%%%%%%%%%%%%%%%%%%%%%%%%%%%%%%%%%%%%%%%%%%%%%%%%%%%%%%

%%%%%%%%%%%%%%%%%%%%%%%%%%%%%%%%%%%%%%%%%%%%%%%%%%%%%%%%%%%%%%%%%%%%%%%%%%%%%%%%%%%%%%%%%%
